# Supplementary material for: Limits of the phonon quasi-particle picture at the cubic-to-tetragonal phase transition in halide perovskites
Source: arXiv:2211.08197 ancillary file (2023-10-07)
Supplement: Supplementary file 1 [file supporting-information.pdf]

## Supplemental Material:

## Limits of the phonon quasi-particle picture at the cubic-to-tetragonal phase transition in halide perovskites

Erik Fransson[1], Petter Rosander[1], Fredrik Eriksson[1], J. Magnus Rahm[1], Terumasa Tadano[2], and Paul Erhart[1]

[1] *Department of Physics, Chalmers University of Technology, SE-41296, Gothenburg, Sweden*
[2] *Research Center for Magnetic and Spintronic Materials, National Institute for Materials Science (NIMS), 1-2-1 Sengen, Tsukuba, Ibaraki 305-0047, Japan*

# Contents

**Supplementary Notes** **2**
S1. Density functional theory calculations . . . . . 2
S2. Training and validation of potential . . . . . 2
S3. Molecular dynamics details . . . . . 5
S4. Force constant expansions . . . . . 5
S5. Self-consistent phonons . . . . . 5
S6. Effective harmonic models from molecular dynamics (MD) . . . . . 5
S7. Phonons and mode projections . . . . . 7

**Supplementary Tables** **12**

**Supplementary References** **12**

# Supplementary Notes

## Supplementary Note S1: Density functional theory calculations

Density functional theory (DFT) calculations were performed using the projector augmented-wave method[1] as implemented in the Vienna ab-initio simulation package[2,3]. To this end, the exchange-correlation contribution was represented using the strongly constrained and appropriately normed (SCAN) density functional[4]. The Brillouin zone was sampled with a Γ-centered grid with a $\boldsymbol{k}$-point density of 0.25 $\text{Å}^{-1}$ and Gaussian smearing with a width of 0.1 eV.

## Supplementary Note S2: Training and validation of potential

A neuroevolution potential (NEP) model was fitted with the GPUMD package (version 3.3.1)[5,6]. The NEP is based on a neural network for which local atomic environments are described by smooth overlap of atomic positions (SOAP)-like descriptors[7] defined in Ref.[8], here with radial and angular cutoff of 8 Å and 4 Å, respectively, and radial and angular order 12 and 6, respectively. The neural network consists of one hidden layer of 40 neurons and a hyperbolic tangent activation function and was trained over 210,000 generations using the natural evolution strategy[9] implemented in GPUMD. Both the $L_1$ and the $L_2$ norm were regularized using $\lambda_1 = \lambda_2 = 0.02$ (as defined in Ref[6]). The model was fitted to forces, energies and virials from DFT calculation of 642 atomic structures with a total of 176 920 atoms, and validated against a set of 72 structures calculated with a total of 19 800 atoms. These structures were generated by means of active learning, i.e., preliminary models were fitted and new structures extracted from MD simulations based on those models were used to fit an updated model.

The model validation against DFT data can be seen in figures Fig. S1, Fig. S2, Fig. S3, Fig. S4. The energy and lattice parameters of the relevant phases are given in Table S1 In Fig. S5 the obtained phonon dispersion from MDs simulations is compared to experimental work[10,11].

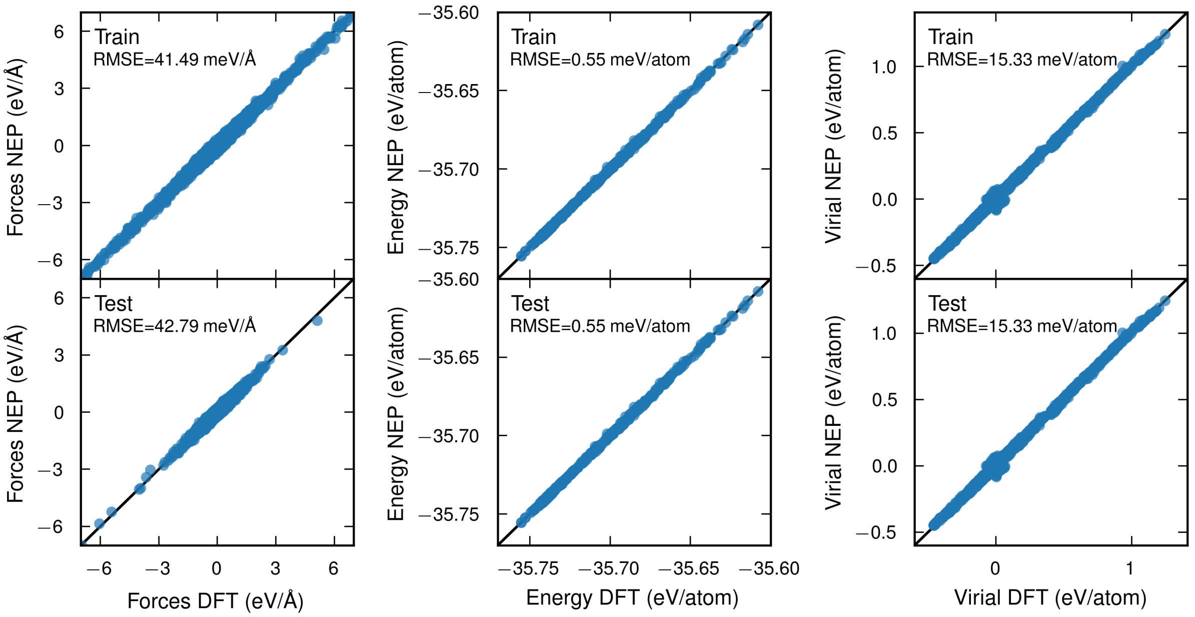


Figure S1: **Parity plots.** Parity plots for energies, forces, and virials for training (top) and test (bottom) data.

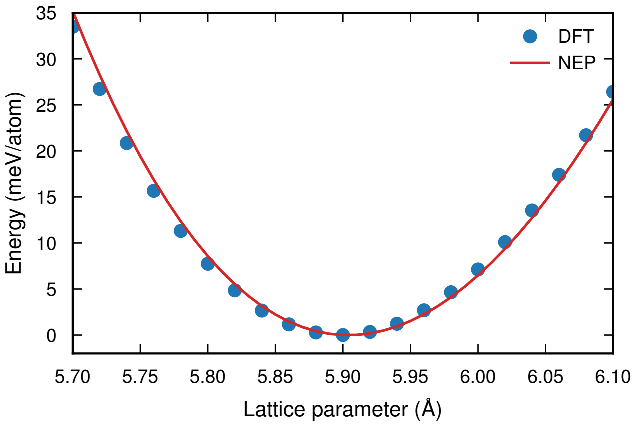


Figure S2: **Energy-volume curves.** Energy-volume curves for the cubic phase of $CsPbBr_3$ from NEP and DFT calculations.

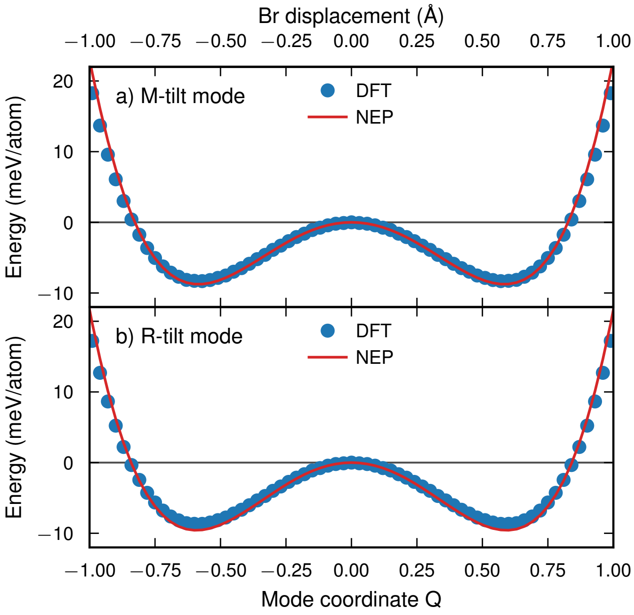


Figure S3: **Energy landscape along phonon modes.** Phonon mode PES along the M and R tilt modes with NEP and DFT. The top x-axis indicates the displacement of each Br atoms involved in the mode in units of Å.

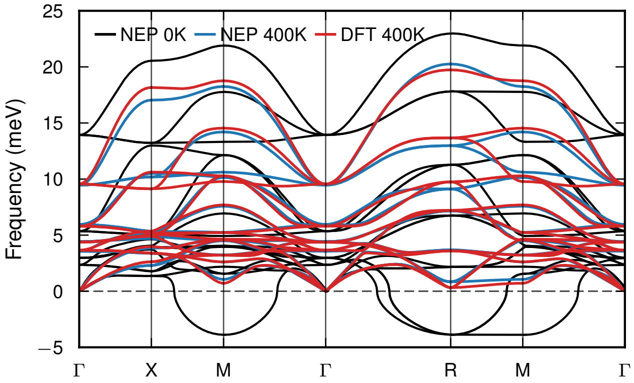


Figure S4: **Phonon dispersion of cubic $CsPbBr_3$.** Phonon dispersions for the cubic phase of $CsPbBr_3$ with the finite temperature dispersions from EHM for DFT and NEP constructed from the same training structures (MD at 400 K).

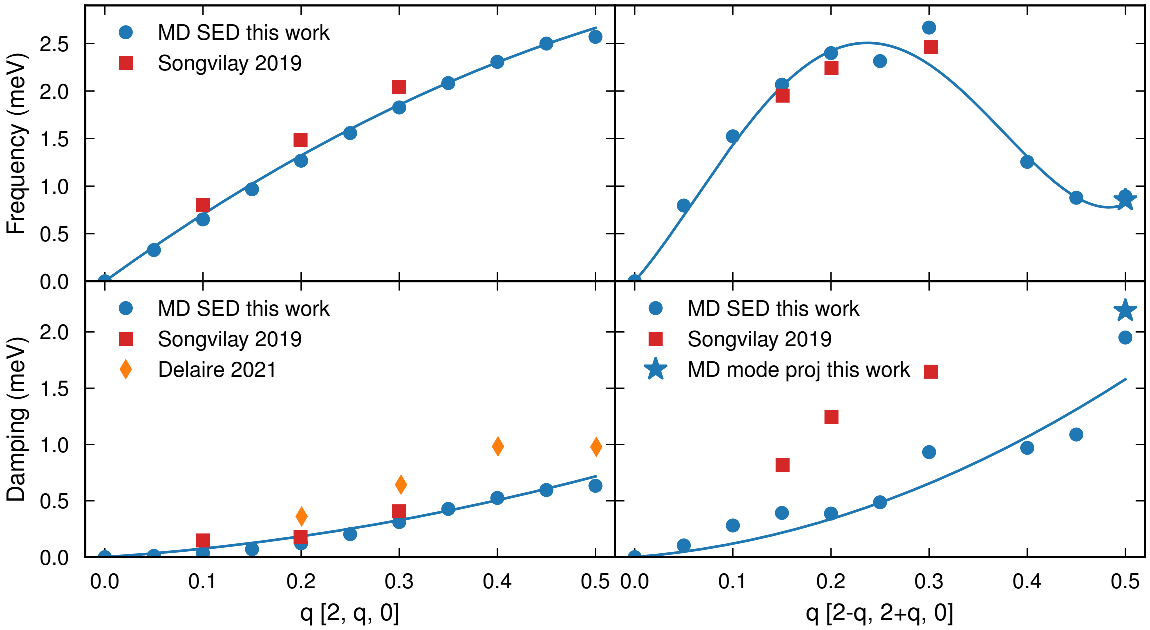


Figure S5: **Phonon dispersion from molecular dynamics compared to experiment.** Phonon frequencies and phonon linewidths for Γ →X (left) and Γ →M (right) calculated using the SED method from MD simulations compared to experimental data[10,11] at 420 K. The point marked with a star correspond to the values obtained through phonon mode-projection. Solid lines serve as guides to the eyes (polynomial fits to the MD data).

## Supplementary Note S3: Molecular dynamics details

The phase transitions were studied with simulated annealing simulations in the isothermal-isobaric ($NpT$) ensemble with a supercell comprising 25 920 atoms. The lattice parameters were extracted for the cubic and tetragonal phases from $NpT$ runs and used in NVT and NVE runs. For all MD simulations a time step of 1 fs was used.

The dynamics of the phonon modes were analyzed via phonon mode projections from MD simulations in the microcanonical ($NVE$) ensemble with a supercell comprising 8640 atoms ($12 \times 12 \times 12$ conventional cubic cells) see Fig. S9 for size convergence. Close to the cubic-tetragonal transition and for the tetragonal phase (see Fig 6) we used larger system sizes upto 400 000 atoms and used supercell size extrapolation (Fig. S10) in order to achieve converged frequencies. For each temperature a total of 50 independent simulations was carried out, each being 1 ns long. Each simulation was first equilibrated for 100 ps in the $NVT$ ensemble, and then the mode coordinate and velocity, Q and P, were recorded in the $NVE$ ensemble every 10th step. The autocorrelation functions (ACFs) of Q and P were calculated for each MD simulation and then were averaged over the 50 independent runs (see Fig. S8 for convergence test).

## Supplementary Note S4: Force constant expansions

The PES can be expanded in a Taylor series in the atomic displacements $\boldsymbol{u}$ relative to a set of reference positions $\boldsymbol{r}_0$

$$U = U_0 + \frac{1}{2}\Phi_{ij}^{\alpha\beta} u_i^\alpha u_j^\beta + \frac{1}{3!}\Phi_{ijk}^{\alpha\beta\gamma} u_i^\alpha u_j^\beta u_k^\gamma + \ldots, \tag{S1}$$

where $\Phi$ are the force constants (FCs), Latin indices enumerate atoms, Greek indices enumerate Cartesian coordinates, and the Einstein summation convention applies.

For all self-consistent phonons (SCP) results temperature specific fourth-order force constant potentials (FCPs) were used. These FCPs were trained from MD simulations with the NEP.

## Supplementary Note S5: Self-consistent phonons

There are several different variations of SCPs[12]. Here, we employ three variants as implemented in ALAMODE[13], SSCHA[14] and HIPHIVE[15].

The SCP implementation in ALAMODE is based on Green's functions.

In the SSCHA scheme the free energy of the harmonic model is minimized,

$$\min_{\mathcal{H}} \left\{ F_{\mathcal{H}} + \langle V - \mathcal{V} \rangle_{\mathcal{H}} \right\}, \tag{S2}$$

where $\mathcal{H}$ the harmonic Hamiltonian and $H$ is the anharmonic Hamiltonian. The first term is thus the harmonic free energy, and the second term is the difference between the harmonic and anharmonic potential evaluated in the harmonic ensemble.

In HIPHIVE a force-fitting SCP is implemented as

$$\min_{\boldsymbol{\Phi}} \left\langle \left( f_i^{\text{har}} - f_i \right)^2 \right\rangle_{\mathcal{H}}, \tag{S3}$$

where $f_i^{\text{har}}$ are the harmonic forces that depend on the harmonic FCs $\boldsymbol{\Phi}$ and $f_i$ are the anharmonic forces. Here, the ensemble average is carried out in the harmonic ensemble, $\mathcal{H}$.

## Supplementary Note S6: Effective harmonic models from MD

Phonon renormalization can also be done by constructing EHMs directly from MD simulations by fitting the harmonic FCs to displacement and force data as follows

$$\min_{\boldsymbol{\Phi}} \left\langle \left( f_i^{\text{har}} - f_i \right)^2 \right\rangle_{H} \tag{S4}$$

This approach has been popularized in the TDEP package[16]. In order to train the EHMs we run MD for a 6×6×6 system in the NVT ensemble (1080 atoms) and select 200 snapshots each separated by 500 fs for each temperature. From these 200 snapshots displacements and forces are extracted and used to fit EHMs with a harmonic cutoff of 9 Å.

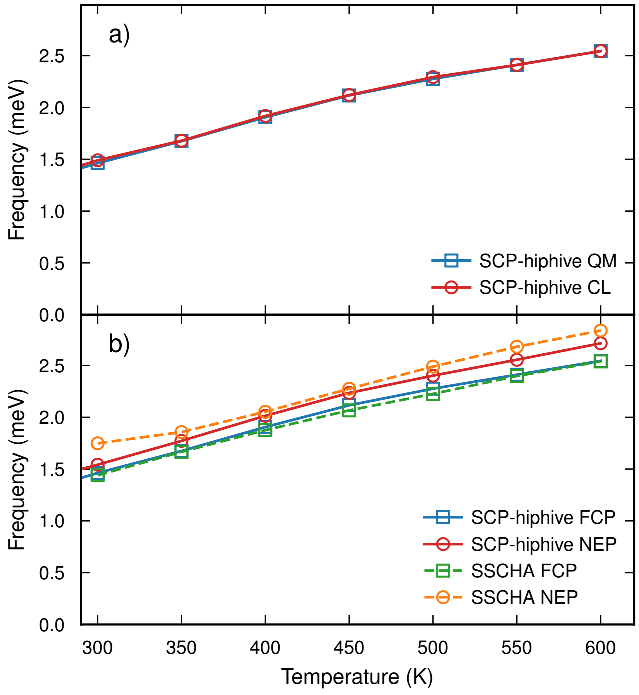


Figure S6: **Self-consistent phonons.** (a) The M-tilt mode frequency vs temperature with the fourth order FCP using SCP-hiphive quantum (QM) and classical (CL) sampling. (b) The M-tilt mode frequency vs temperature with compared between fourth-order FCP and using the NEP model directly.

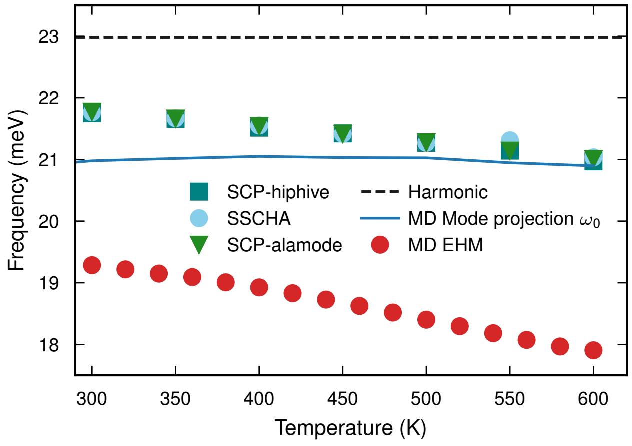


Figure S7: **Frequency of optical mode.** Temperature dependent frequency for the highest optical mode at R with different methods.

## Supplementary Note S7: Phonons and mode projections

Below some more details and convergence tests are shown for the phonon mode projections. Convergence with respect to simulation time is shown in Fig. S8 and with respect to system size Fig. S9. The size-extrapolation of the phonon frequency and lifetimes are shown in Fig. S10.

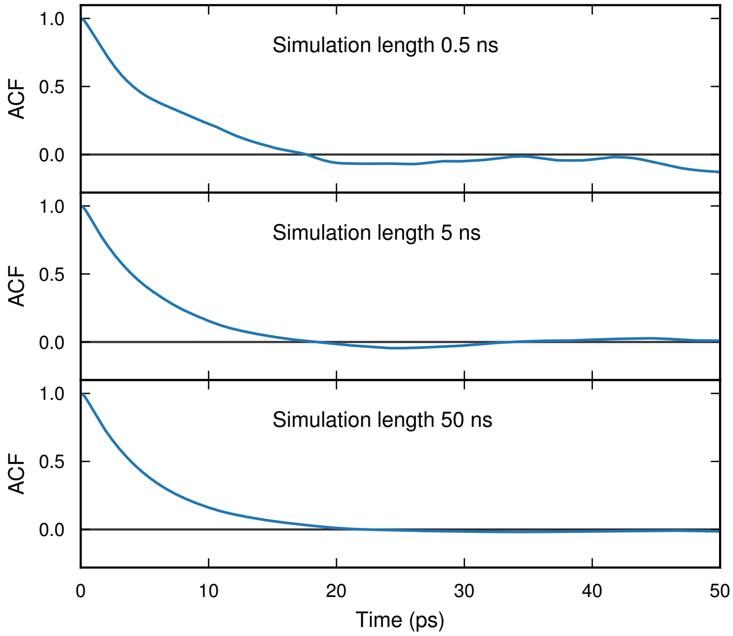


Figure S8: **Auto-correlation functions convergence with respect to simulation length.** The ACF, $C_Q(t)$, of the M-tilt mode at 350 K with different total number of time steps considered in the ensemble averaging. A well converged ACF is obtained for 50 ns.

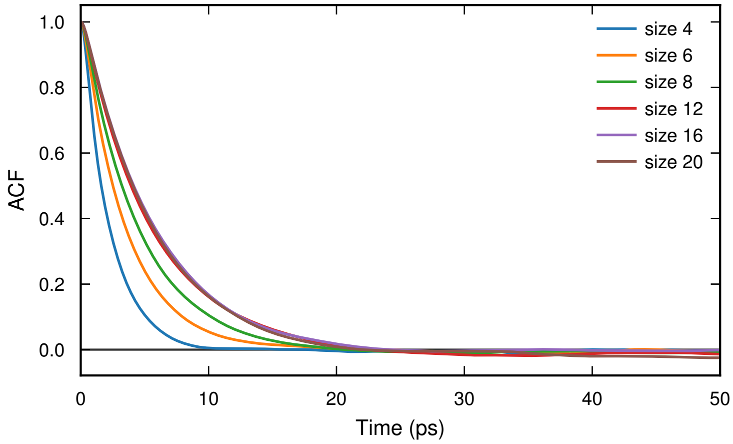


Figure S9: **Auto-correlation functions convergence with respect to system size.** The ACF, $C_Q(t)$, of the M-tilt mode at 350 K for different system size (size $N$ refers to a supercell of $N \times N \times N$ conventional cubic cells). Here, the sizes 12, 16, 20 produce almost identical ACFs.

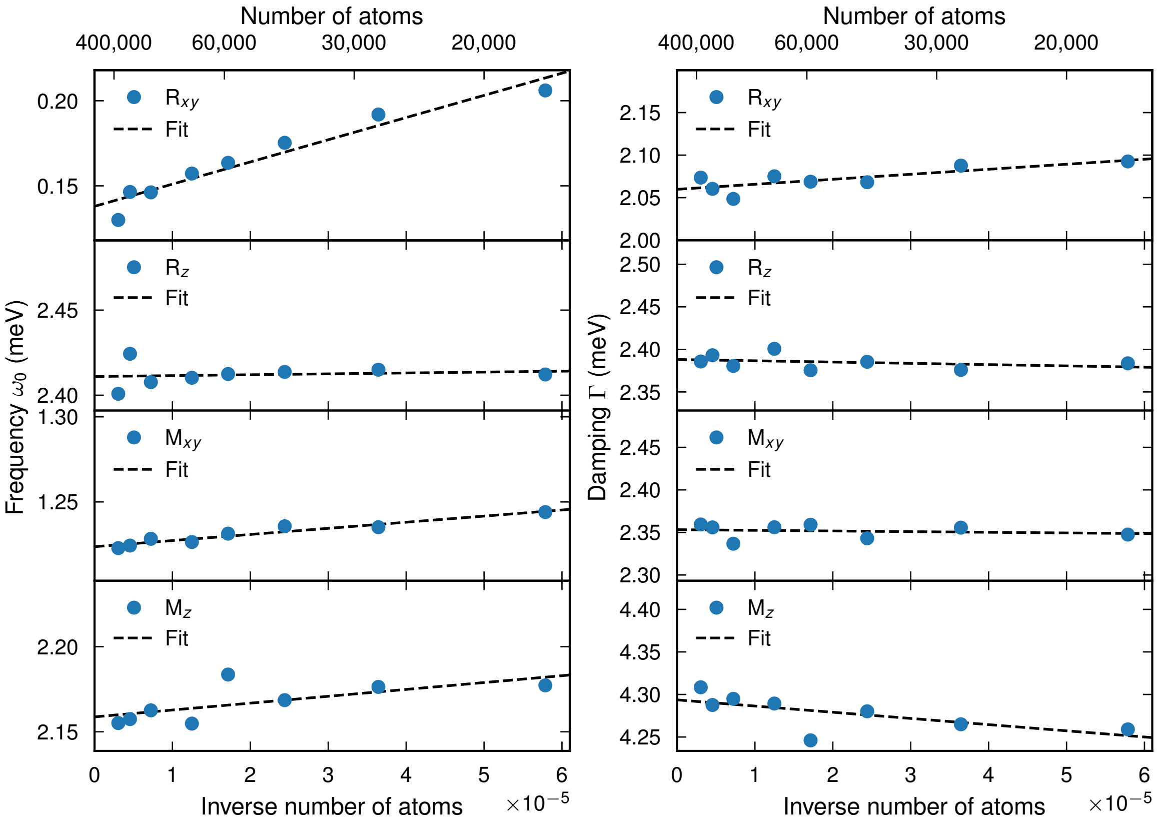


Figure S10: **System size dependency of frequency and damping.** The frequencies, $\omega_0$ and damping, $\Gamma$, obtained from fitting the ACFs to a DHO for the different modes in the tetragonal structure for various system sizes at 276 K. The solid lines correspond to linear fits, from which the infinte system size extrapolated values can be extracted. The frequency of the $R_{xy}$ mode shows a strong size dependency, specially for temperatures close to the orthorhombic transition. The dampings, $\Gamma$, do not appear to be very sensitive to system size for any temperature.

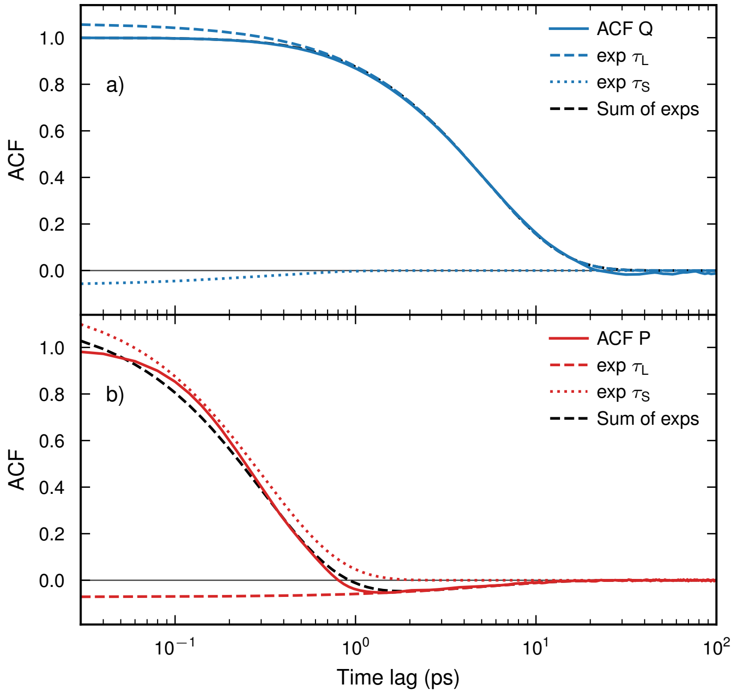


Figure S11: **Decomposition of auto-correlation functions.** (a) The ACF of the mode coordinate, $C_Q(t)$, of the M-tilt mode at 350 K. (b) The ACF of the mode velocity, $C_P(t)$, of the M-tilt mode at 350 K. The timescales are $\tau_\mathrm{L}$ =5.22 ps and $\tau_\mathrm{S}$ =0.31 ps. Here, the solid lines corresponds to the raw ACF obtained from MD, the black dashed line corresponds to the fitted DHO, the colored dashed line corresponds to the long-timescale exponential decay in of the overdamped DHO and the dotted line corresponds to the short-time scale exponential decay.

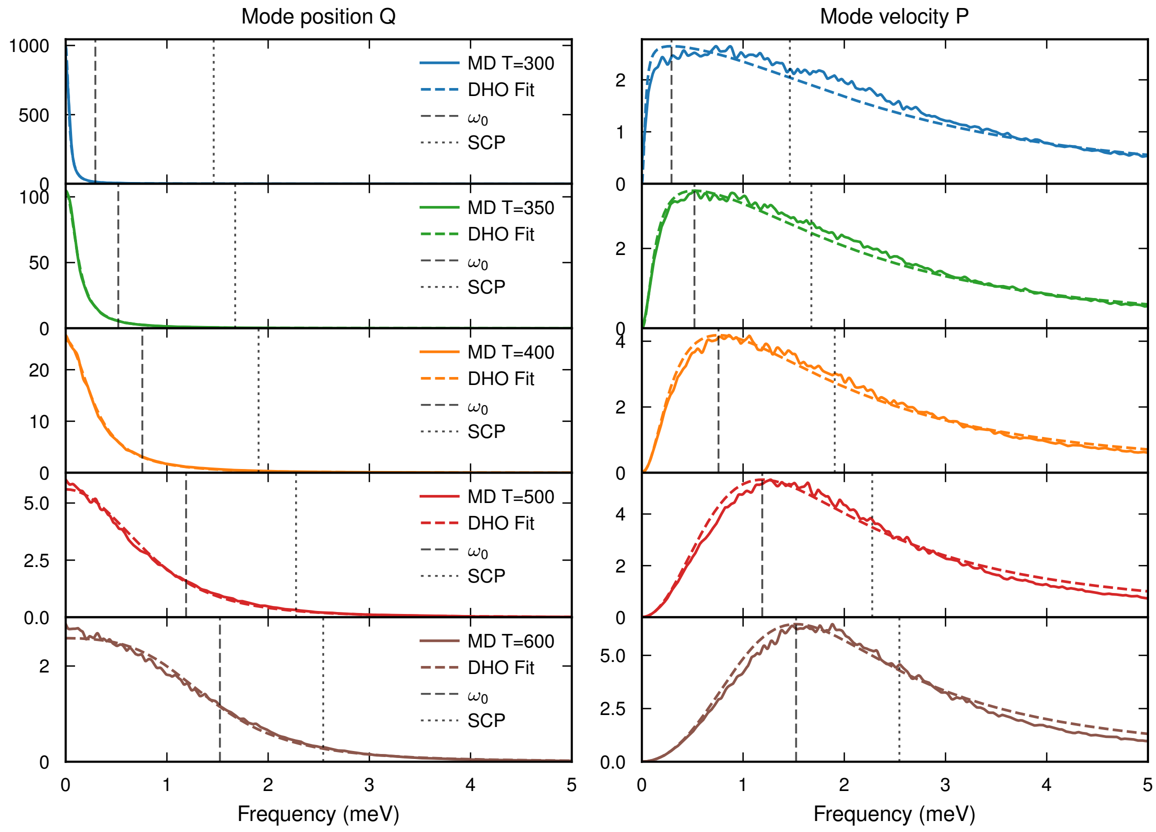


Figure S12: **Phonon mode powerspectra.** Power spectra of the M-tilt mode at various temperatures for the position ($Q$) and velocity ($P$) of the mode. The solid lines are the raw spectra obtained from MD simulations, the dashed colored lines correspond to the fits to the DHO, the dashed vertical lines correspond to $\omega_0$ from the DHO and the dotted lines correspond to the frequency obtained from SCP.

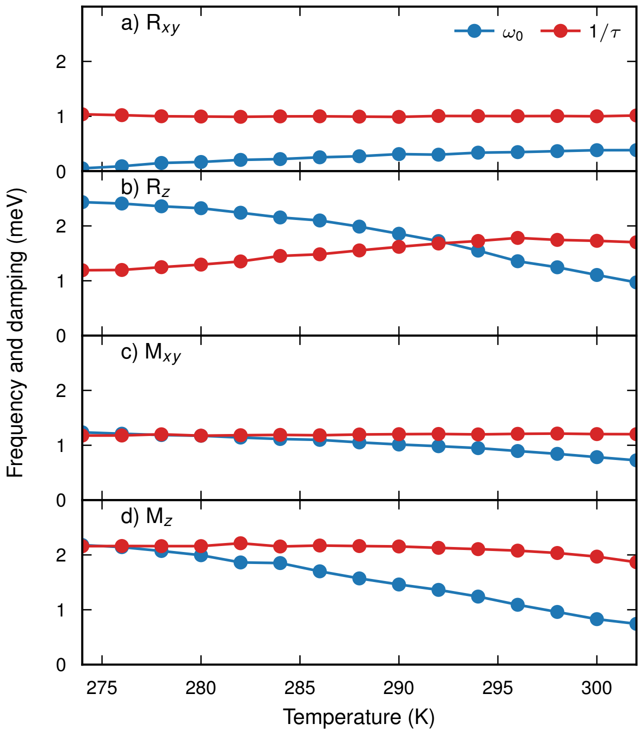


Figure S13: **Phonon frequencies and lifetimes in the tetragonal phase.** Phonon frequencies $\omega_0$ and relaxation time $\tau$ in the tetragonal phase obtained from MD simulations for the modes a) $R_{xy}$, b) $R_z$, c) $M_{xy}$, and d) $M_z$, respectively.

# Supplementary Tables

Table S1: Comparison of structural parameters of the orthorhombic, tetragonal and cubic phase between NEP and DFT.

| | Spacegroup | Energy (meV/atom) | $a$ (Å) | $b$ (Å) | $c$ (Å) |
|---|---|---|---|---|---|
| NEP | | | | | |
| cubic | Pm$\bar{3}$m (221) | 17.589 | 5.9042 | | |
| tetragonal | P4/mbm (127) | 4.659 | 5.7883 | | 5.9791 |
| orthorhombic | Pnma (62) | 0.0 | 5.6388 | 5.8751 | 5.9996 |
| DFT (SCAN) | | | | | |
| cubic | Pm$\bar{3}$m (221) | 14.647 | 5.8987 | | |
| tetragonal | P4/mbm (127) | 3.753 | 5.7788 | | 5.9852 |
| orthorhombic | Pnma (62) | 0.0 | 5.7032 | 5.8682 | 5.9451 |

# Supplementary References


[1] P. E. Blöchl. Projector augmented-wave method. *Physical Review B*, 50:17953–17979, 1994. doi: 10.1103/PhysRevB.50.17953.

[2] G. Kresse and J. Hafner. Ab initio molecular dynamics for liquid metals. *Physical Review B*, 47: 558–561, Jan 1993. doi: 10.1103/PhysRevB.47.558.

[3] G. Kresse and J. Furthmüller. Efficiency of ab-initio total energy calculations for metals and semiconductors using a plane-wave basis set. *Computational Materials Science*, 6(1):15–50, 1996. doi: 10.1016/0927-0256(96)00008-0.

[4] Jianwei Sun, Adrienn Ruzsinszky, and John P. Perdew. Strongly Constrained and Appropriately Normed Semilocal Density Functional. *Physical Review Letters*, 115:036402, Jul 2015. doi: 10.1103/PhysRevLett.115.036402.

[5] Zheyong Fan, Topi Siro, and Ari Harju. Accelerated molecular dynamics force evaluation on graphics processing units for thermal conductivity calculations. *Computer Physics Communications*, 184(5):1414–1425, 2013. ISSN 0010-4655. doi: doi.org/10.1016/j.cpc.2013.01.008. URL `https://www.sciencedirect.com/science/article/pii/S0010465513000258`.

[6] Zheyong Fan, Zezhu Zeng, Cunzhi Zhang, Yanzhou Wang, Keke Song, Haikuan Dong, Yue Chen, and Tapio Ala-Nissila. Neuroevolution machine learning potentials: Combining high accuracy and low cost in atomistic simulations and application to heat transport. *Physical Review B*, 104: 104309, Sep 2021. doi: 10.1103/PhysRevB.104.104309. URL `https://link.aps.org/doi/10.1103/PhysRevB.104.104309`.

[7] Albert P. Bartók, Risi Kondor, and Gábor Csányi. On representing chemical environments. *Physical Review B*, 87:184115, May 2013. doi: 10.1103/PhysRevB.87.184115. URL `https://link.aps.org/doi/10.1103/PhysRevB.87.184115`.

[8] Zheyong Fan. Improving the accuracy of the neuroevolution machine learning potential for multi-component systems. *Journal of Physics: Condensed Matter*, 34(12):125902, jan 2022. doi: 10.1088/1361-648x/ac462b. URL `https://doi.org/10.1088/1361-648x/ac462b`.

[9] Daan Wierstra, Tom Schaul, Tobias Glasmachers, Yi Sun, Jan Peters, and Jürgen Schmidhuber. Natural evolution strategies. *Journal of Machine Learning Research*, 15(27):949–980, 2014. URL `http://jmlr.org/papers/v15/wierstra14a.html`.

[10] M. Songvilay, N. Giles-Donovan, M. Bari, Z.-G. Ye, J. L. Minns, M. A. Green, Guangyong Xu, P. M. Gehring, K. Schmalzl, W. D. Ratcliff, C. M. Brown, D. Chernyshov, W. van Beek, S. Cochran, and C. Stock. Common acoustic phonon lifetimes in inorganic and hybrid lead halide perovskites. *Physical Review Materials*, 3:093602, Sep 2019. doi: 10.1103/PhysRevMaterials.3.093602. URL `https://link.aps.org/doi/10.1103/PhysRevMaterials.3.093602`.

[11] Tyson Lanigan-Atkins, Xing He, MJ Krogstad, DM Pajerowski, DL Abernathy, Guangyong NMN Xu, Zhijun Xu, D-Y Chung, MG Kanatzidis, Stephana Rosenkranz, R. Osborn, and O. Delaire. Two-dimensional overdamped fluctuations of the soft perovskite lattice in CsPbBr3. *Nature Materials*, 20(7):977–983, 2021. doi: 10.1038/s41563-021-00947-y.

[12] Keivan Esfarjani and Yuan Liang. Thermodynamics of anharmonic lattices from first principles. In *Nanoscale Energy Transport*, 2053-2563, pages 7–1 to 7–35. IOP Publishing, Bristol England, 2020. ISBN 978-0-7503-1738-2. doi: 10.1088/978-0-7503-1738-2ch7. URL `http://dx.doi.org/10.1088/978-0-7503-1738-2ch7`.

[13] T. Tadano, Y. Gohda, and S. Tsuneyuki. Anharmonic force constants extracted from first-principles molecular dynamics: applications to heat transfer simulations. *Journal of Physics: Condensed Matter*, 26(22):225402, 2014. ISSN 0953-8984. doi: 10.1088/0953-8984/26/22/225402.

[14] Lorenzo Monacelli, Raffaello Bianco, Marco Cherubini, Matteo Calandra, Ion Errea, and Francesco Mauri. The stochastic self-consistent harmonic approximation: calculating vibrational properties of materials with full quantum and anharmonic effects. *Journal of Physics: Condensed Matter*, 33(36):363001, jul 2021. doi: 10.1088/1361-648x/ac066b.

[15] Fredrik Eriksson, Erik Fransson, and Paul Erhart. The Hiphive Package for the Extraction of High-Order Force Constants by Machine Learning. *Advanced Theory and Simulations*, 2:1800184, 2019. ISSN 2513-0390. doi: 10.1002/adts.201800184. URL `https://onlinelibrary.wiley.com/doi/abs/10.1002/adts.201800184`.

[16] Olle Hellman, Peter Steneteg, I. A. Abrikosov, and S. I. Simak. Temperature dependent effective potential method for accurate free energy calculations of solids. *Physical Review B*, 87(10):104111, March 2013. doi: 10.1103/PhysRevB.87.104111.
